# Supplementary material for: Evolution of the structural transition in Mo$_{1-x}$W$_{x}$Te$_{2}$
Source: arXiv:2003.08531 source file (2020-06-11)
Supplement: Supplementary file 1 [file supplement.pdf]

# Supplemental Materials: Exploration of the $\text{Mo}_{1-x}\text{W}_x\text{Te}_2$ structural phase transition

John A. Schneeloch,<sup>1</sup> Yu Tao,<sup>1</sup> Chunruo Duan,<sup>1,\*</sup> Masaaki Matsuda,<sup>2,†</sup> Adam A. Aczel,<sup>2,3,†</sup> Jaime A. Fernandez-Baca,<sup>2,†</sup> Guangyong Xu,<sup>4</sup> Jörg C. Neuefeind,<sup>2,†</sup> Junjie Yang,<sup>1,‡</sup> and Despina Louca<sup>1,§</sup>

<sup>1</sup>*Department of Physics, University of Virginia, Charlottesville, Virginia 22904, USA*

<sup>2</sup>*Neutron Scattering Division, Oak Ridge National Laboratory, Oak Ridge, Tennessee 37831, USA*

<sup>3</sup>*Department of Physics and Astronomy, University of Tennessee, Knoxville, Tennessee 37996, USA*

<sup>4</sup>*NIST Center for Neutron Research, National Institute of Standards and Technology, Gaithersburg, Maryland 20877, USA*

## LATTICE PARAMETERS

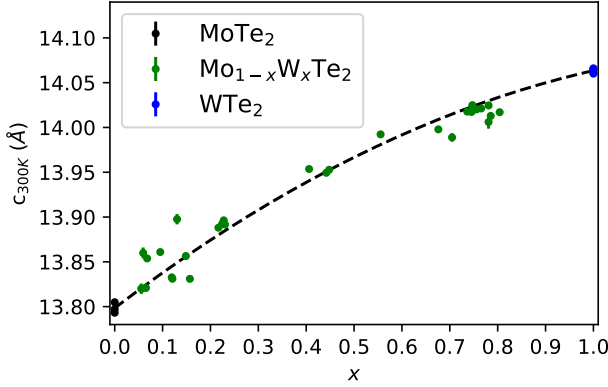

FIG. S1. Relationship between  $c$ , obtained at room temperature from  $(00L)$  Bragg peak positions in XRD scans of single crystals, and W fraction  $x$ , estimated from EDS measurements. The dashed line represents a quadratic fitting of the data points, fixed at the endpoints to the mean  $c_{300\text{K}}$  values for  $\text{MoTe}_2$  and  $\text{WTe}_2$ . Only errorbars for  $c_{300\text{K}}$  are shown; error in  $x$  is suggested by the scatter.

Since the EDS-estimated W-fractions of  $\text{Mo}_{1-x}\text{W}_x\text{Te}_2$  crystals grown by flux growth often differ substantially from the nominal  $x$ , we chose to characterize the W-fraction via  $c_{300\text{K}}$ , the value of  $c$  at 300 K. This method allows us to characterize samples by a quantity determined from the same aligned crystal domain as that used to obtain the rest of the neutron scattering data.

To determine the relationship between  $x$  and  $c_{300\text{K}}$  (and to complement relationships reported in the literature [1, 2]), we used X-ray diffraction (XRD) to obtain  $c$  from  $(00L)$  scans, and used EDS on the same samples to estimate the W-fraction. Scans of  $\theta$ - $2\theta$  were conducted on a powder X-ray diffractometer in the Bragg-Brentano geometry to obtain the  $2\theta$  positions of the  $(00L)$  peaks up to  $L = 8$ . These  $(00L)$  peak positions were fit to Bragg's law plus a correction for specimen displacement error. This error, which comes from the sample not being positioned perfectly on the focusing circle of the goniometer, is estimated as  $\delta(2\theta) = -2s(\cos \theta/R)$ , where  $s$  is the displacement of the specimen from the focusing circle of radius  $R$  [3]. These measurements were all performed at room temperature.

Fig. S1 displays the  $c_{300\text{K}}$  and  $x$  values determined by XRD and EDS. The low spread in  $c_{300\text{K}}$  for  $\text{MoTe}_2$  and  $\text{WTe}_2$  suggest that most of the scatter seen in Fig. S1 is due to uncertainty in the EDS determination of  $x$  (presumably due to inhomogeneity), rather than uncertainty in the determination of  $c$ . A monotonic increase of  $c$  with  $x$  can be seen. A quadratic curve was fitted through the data, kept fixed at the mean values for  $\text{MoTe}_2$  and  $\text{WTe}_2$ . This quadratic relation was used to convert  $c_{300\text{K}}$  obtained from neutron scattering scans across  $(004)$  to the effective values of  $x$  shown in Table I in the main text. (For MWT3, we instead deduced  $c_{300\text{K}}$  from the distance between the  $(202)$  and  $(203)$   $T_d$ -phase Bragg peaks. To account for systematic error due to deriving  $c_{300\text{K}}$  from the distance between  $(202)$  and  $(203)$  rather than the position of  $(004)$ , the difference in  $c_{300\text{K}}$  obtained from these two methods for MWT1 was determined and used to adjust the value obtained for MWT3. For MWT7, we used a value measured at 300 K for  $c_{300\text{K}}$  rather than extrapolating from other temperatures.)

The temperature-dependence of  $c$  for the crystals studied by neutron scattering was obtained both to determine  $c_{300\text{K}}$  and for insight into structural differences as a function of W-substitution. These data are shown in Fig. S2(a). The values of  $c$  were determined from the position of the  $(004)$  peak in longitudinal neutron scattering scans; data were taken on SPINS and HB1A. A linear fit to data closest to 300 K was used to obtain  $c_{300\text{K}}$ . Though only one Bragg peak was used to determine  $c$ , the similar  $c$  values for MT1, MT2, and MT3 suggest that systematic errors resulted in a random deviation of  $c$  on the order of  $\sim 0.01$  Å.

Some data, such as for MWT1, show kinks in the

\* Present address: Department of Physics and Astronomy, Rice University, Houston, Texas 77005, USA

† Notice: This manuscript has been authored by UT-Battelle, LLC, under contract DE-AC05-00OR22725 with the US Department of Energy (DOE). The US government retains and the publisher, by accepting the article for publication, acknowledges that the US government retains a nonexclusive, paid-up, irrevocable, worldwide license to publish or reproduce the published form of this manuscript, or allow others to do so, for US government purposes. DOE will provide public access to these results of federally sponsored research in accordance with the DOE Public Access Plan (<http://energy.gov/downloads/doe-public-access-plan>).

‡ Present address: Department of Physics, New Jersey Institute of Technology, University Heights, Newark, New Jersey 07102

§ Corresponding author; louca@virginia.edu

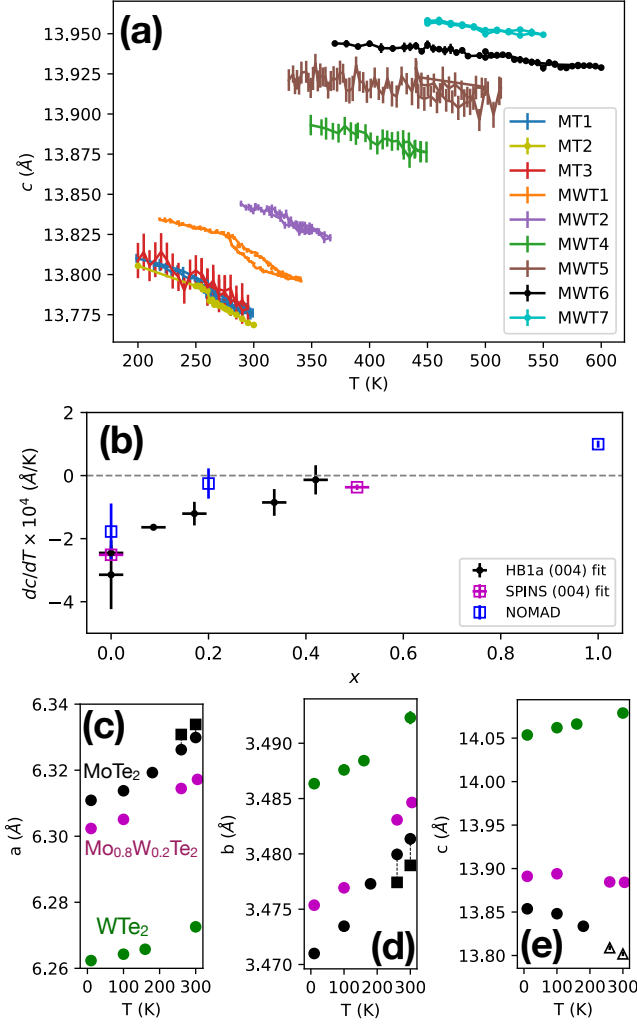

FIG. S2. (a) The temperature-dependence of  $c$  obtained from the position of (004) from fits to longitudinal scans. (b) Estimates of the slope  $dc/dT$  at 300 K as a function of  $x$ . (c-e) Lattice constants  $a$ ,  $b$ , and  $c$  obtained from refinement of neutron powder diffraction data taken on NOMAD. Circles and squares denote T<sub>d</sub>- and 1T'-phase fits, respectively. Triangles denote  $c$  obtained from fits to the (002) peak.

temperature-dependence of  $c$  corresponding to structural transitions. These kinks are likely due to a slight misalignment occurring during the transition; for example, the (004) peak was observed to move slightly in the angular direction during the transition of MWT1. Combined with the anisotropy of the neutron scattering resolution function, this misalignment could be responsible for the apparent shift of the (004) position and thus  $c$ .

Thermal contraction is an unusual property, even more notable in Mo<sub>1-x</sub>W<sub>x</sub>Te<sub>2</sub> since the structurally similar MoTe<sub>2</sub> and WTe<sub>2</sub> behave oppositely. Fig. S2(b) shows quantitatively the change in  $dc/dT$  from the  $c$ -axis thermal contraction of MoTe<sub>2</sub> to the (more conventional)  $c$ -axis thermal expansion of WTe<sub>2</sub>. For each crystal (and

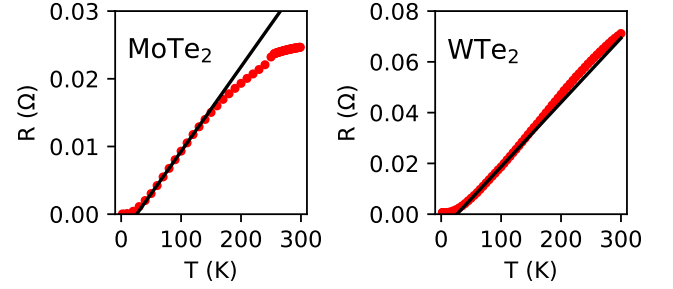

FIG. S3. Resistance along the  $b$ -axis of MoTe<sub>2</sub> and WTe<sub>2</sub>, taken on cooling. The black lines represent linear fits to data within  $50 \leq T \leq 100$  K.

for powders measured on NOMAD, to be discussed below), values of  $dc/dT$  were determined by extrapolating from points in the T<sub>d</sub> phase nearest to 300 K. The data suggest a gradual change from negative to positive  $c$ -axis thermal expansion with increased W substitution.

Data taken on NOMAD were also used to determine the temperature-dependence of lattice constants, as shown in Fig. S2(c-e). All NOMAD data were taken on cooling from the highest temperature. Refinement was done in the T<sub>d</sub> phase for all temperatures of WTe<sub>2</sub> and Mo<sub>0.8</sub>W<sub>0.2</sub>Te<sub>2</sub>, and for the lower temperatures (10 K, 100 K, and 180 K) of MoTe<sub>2</sub>. For MoTe<sub>2</sub> at 260 K and 300 K, the diffraction pattern appeared to show substantial diffuse scattering, so refinement was done for a mixture of the 1T' and T<sub>d</sub> phases. Thus, in Figures S2(c) and S2(d), the  $a$  and  $b$  lattice parameters for both refined phases are shown, which illustrate a likely range in which the true  $a$  and  $b$  values reside. For  $c$ , the fact that the (002) peak was isolated from the other peaks allowed the (002) position to be fitted to determine  $c$ . We accounted for a systematic error between  $c$  deduced from the position of (002) and the refined  $c$  by calculating the systematic error present at 180, 100, and 10 K (about  $\sim 0.025$  Å) and adjusting the 260 and 300 K (002)-derived  $c$  values accordingly.

The nearly linear increase in  $c$  for WTe<sub>2</sub> in Fig. S2(e) is striking compared to the downward curvature of  $c$  for MoTe<sub>2</sub>. Transport properties differ similarly. The temperature-dependence of the resistance (Fig. S3) is nearly linear in  $T$  for WTe<sub>2</sub> but has a downward curvature for MoTe<sub>2</sub>. The Hall coefficient is reported to be nearly flat above  $\sim 50$  K for WTe<sub>2</sub> [4, 5], but continually changing for MoTe<sub>2</sub> [6–8]. The chemical potential  $\mu(T)$  also appears to behave differently, moving in opposite directions for WTe<sub>2</sub> and MoTe<sub>2</sub> (as deduced from the Lifshitz transition in WTe<sub>2</sub> [4, 5] and optical conductivity measurements in MoTe<sub>2</sub> [9], and consistent with the expectation that the chemical potential moves toward a lower density of states with increased temperature [9] given calculated densities of states as a function of energy for WTe<sub>2</sub> [5, 10, 11] and MoTe<sub>2</sub> [9, 11].) Fur-

ther research should clarify possible connections between the divergence in structural and electronic properties between  $\text{WTe}_2$  and  $\text{MoTe}_2$ .

### UNUSUALLY BROAD TRANSITIONS IN $\text{MoTe}_2$

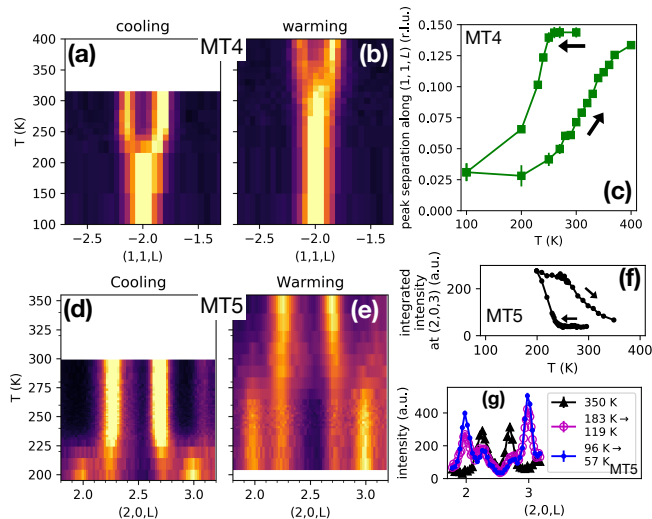

FIG. S4. (a,b) Neutron scattering intensity along  $(1, 1, L)$  as a function of temperature on cooling, then warming. Data taken on a nominally  $\text{MoTe}_2$  crystal, labeled MT4, at SPINS at the NCNR. Intensity near  $L = 3.1$  and  $L = 2.4$  are from  $\text{MoTe}_2$  powder lines from and  $(11\bar{3})_{1T'}$  and  $(013)_{1T'}$ , respectively. (c) Fitted separation between the two peaks about  $L = -2$ . (d,e) Neutron scattering intensity on a different  $\text{MoTe}_2$  crystal, MT5, plotted as intensity along  $(2, 0, L)$  as a function of temperature. Data taken on HB1 at HFIR. (f) Intensity of the data in (d,e) averaged within  $2.92 \leq L \leq 3.08$ . (g) Individual scans along  $(2, 0, L)$  for MT5, first at 350 K, and then on cooling down to 57 K. Due to a heater malfunctioning, this cooling was uncontrolled, during which points were measured in order of increasing  $L$  within the ranges shown in the legend.

For two nominally  $\text{MoTe}_2$  crystals, which we refer to as MT4 and MT5, transition over much broader temperature ranges were observed than for our other  $\text{MoTe}_2$  or  $\text{Mo}_{1-x}\text{W}_x\text{Te}_2$  crystals, whose transitions occurred within  $\sim 40$  K.

For the MT4 crystal, intensity along  $(1, 1, L)$  as a function of temperature on cooling and warming is shown in Fig. S4(a,b). At higher temperatures, the two peaks observed are  $(11\bar{2})_{1T'}$  and  $(112)_{1T'}$ , while the  $(11\bar{2})_{Td}$  peak is seen at lower temperatures. To parameterize the transition, we fitted individual intensity vs.  $(1, 1, L)$  scans with two Gaussian peaks with equal widths and an equal distance about  $L = -2$ . The distance along  $L$  between these peaks is plotted in Fig. S4(c). The onset of the transition into  $T_d$  is  $\sim 250$  K, and change continues gradually down to at least 200 K. On warming, the fitted

peak separation increases gradually from 200 K, and did not fully increase to its initial value by 400 K.

For the MT5 crystal, intensity along  $(2, 0, L)$  as a function of temperature is plotted in Fig. S4(d,e). Intensity averaged near  $L = 3$  is plotted in Fig. S4(f) to characterize the transition. On cooling, the onset of the transition into  $T_d$  starts below  $\sim 240$  K (far lower than the  $\sim 280$  K transition onset in the MT1 or MT2 crystals in Fig. 5(a) of the main text), but phase coexistence remains by 200 K. On warming, a slight decrease in intensity near  $L = 3$  is seen, followed by a steeper descent starting around 260 K, though the transition back to  $1T'$  does not complete even up to 350 K. On subsequently cooling below  $\sim 100$  K,  $1T'$  peaks near  $L = 2.3$  and  $L = 2.7$  are still seen in Fig. S4(g), though with reduced intensity.

Both of these nominally  $\text{MoTe}_2$  crystals have unusually broad transitions. A possible cause is Te vacancies, which have been reported to broaden the transition [8], though EDS measurements were inconclusive, indicating vacancies in MT4 but not MT5, with Te:Mo ratios of 1.88(5) and 1.98(3), respectively. (EDS is not perfectly reliable as an indicator of composition; among other reasons, it is only sensitive to the outer surface of crystals.) If Te vacancies exist in MT4 or MT5, they may have been introduced during the post-annealing process, where the Te flux was removed from around  $\text{Mo}_{1-x}\text{W}_x\text{Te}_2$  crystals by heating in an evacuated ampoule back up to 900-1000  $^\circ\text{C}$  in a tube furnace with one end of the ampoule stuck outside, then decanting the Te flux toward the cold end. If the post-annealing were performed for too long, beyond the point at which elemental Te is fully evaporated, then the crystal could start to lose Te. Other possible explanations for the broadened transition include oxygen or moisture, which are conjectured to stabilize the  $1T'$  phase in thin  $\text{MoTe}_2$  crystals [12]. More generally, structural defects may have a similar influence on the transition as stress (either hydrostatic or non-hydrostatic pressure [13], or applied strain [14]) or thickness (sufficiently thin crystals of  $\text{MoTe}_2$  are also reported to have a broadened transition [15].)

### ADDITIONAL NEUTRON SCATTERING DATA

In this section, we present additional neutron scattering data beyond that shown in the main text. Fig. S5 shows data combined from scans of intensity along  $(2, 0, L)$  at various temperatures on warming and cooling through a hysteresis loop. Fig. S5 (a,b), (c,d) and (e,f) show data taken at ambient pressure for MT3, MWT3 and MWT6, respectively. These figures complement the data in Fig. 2 in the main text.

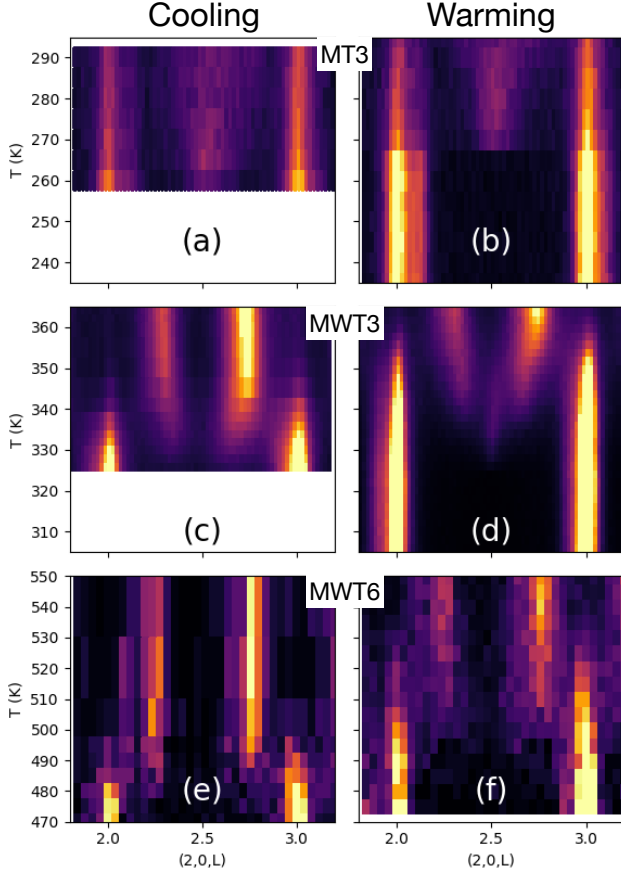

FIG. S5. Neutron scattering intensity along  $(2, 0, L)$  as a function of temperature on (a,c,e) cooling and (b,d,f) warming, on the (a,b) MT3, (c,d) MWT3 and (e,f) MWT6 crystals. Data taken at HB1A for MT3, MWT3 and SPINS for MWT6. For MT3 and MWT3, data were taken on warming, then cooling. For MWT6, data was taken on cooling, then warming. Due to limitations of the sample environment, MT3 could not be warmed above 300 K.

### SIMULATIONS OF STACKING DISORDER IN $\text{MOTe}_2$

Here, we show via simulations that  $T_d^*$ -like transitions in  $1T'$  (e.g.,  $\text{BABABA} \rightarrow \text{BAABBA}$ ) tend to move the  $1T'$  Bragg peaks near  $(2, 0, 2.3)$  and  $(2, 0, 2.7)$  toward  $L = 2.5$ , while  $T_d$ -like transitions in  $1T'$  (e.g.,  $\text{ABABAB} \rightarrow \text{ABAAAB}$ ) tend to move these  $1T'$  peaks away from  $L = 2.5$ . In Fig. S6, we show simulated elastic neutron scattering along  $(2, 0, L)$  for two different models of stacking disorder that might occur on cooling from  $1T'$ . For each of these models, diffuse scattering along  $(2, 0, L)$  was computed by calculating the structure factor of points along this line for a supercell of 16000  $\text{MoTe}_2$  layers, with the model determining how the A/B stacking deviates from the ABAB... stacking of  $1T'$ . The intralayer atomic positions were taken from those reported in Ref. [16] for the  $T_d$  phase. Both models start from a

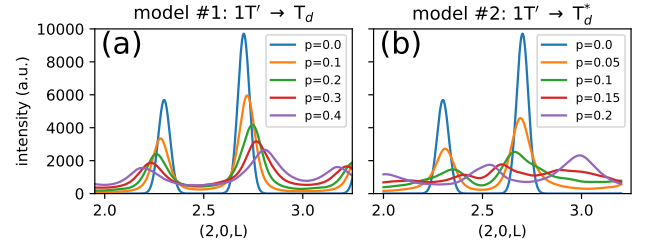

FIG. S6. Simulated neutron scattering intensity along  $(2, 0, L)$ .

50%/50% mixture of the two  $1T'$  twins.

In model #1, starting from the ABAB... stacking, each B-type interlayer boundary has a probability  $p$  of “flipping” from B→A, bringing  $1T'$  closer to  $T_d$  as  $p$  increases. (For example,  $\text{ABABAB} \dots \rightarrow \text{ABAAAB} \dots$ ) From Fig. S6(a), we see that, on increasing  $p$  (in the range of  $p \leq 0.2$ ), diffuse scattering increases and Bragg peak intensity decreases, and the Bragg peaks shift away from  $L = 2.5$  and toward the  $T_d$  Bragg peak locations of  $L = 2$  and  $L = 3$ .

In model #2, starting from the ABAB... stacking, flips of pairs of neighboring sites occur, either  $\text{BABA} \rightarrow \text{BBAA}$  or  $\text{ABAB} \rightarrow \text{AABB}$ , with the locations of the BABA or ABAB blocks chosen at random, and with flipping continuing until a fraction  $p \times 16000$  of flips occur. From Fig. S6(b), we see that for model #2, intensity moves toward  $L = 2.5$ , rather than away from  $L = 2.5$  as it does for model #1.

Thus, movement of the  $1T'$  Bragg peaks toward  $L = 2.5$  on cooling suggest the presence of coordinated  $\text{AB} \rightarrow \text{BA}$ -type shifts bringing  $1T'$  closer to  $T_d^*$ , rather than individual  $\text{A} \rightarrow \text{B}$  shifts that would be a more direct path from  $1T'$  to  $T_d$ .

### TEMPERATURE-DEPENDENCE OF INTENSITY NEAR $(2, 0, 2.5)$

In Fig. S7, we show the temperature-dependence of neutron scattering intensity averaged near  $(2, 0, 2.5)$ , which complements the intensities averaged near  $(2, 0, 3)$  shown in Fig. 4(a,b) in the main text. For crystals with lower W-fraction (MT1, MT2, MT3, MWT1, MWT2, and MWT3), on warming, the intensity near  $(2, 0, 2.5)$  increases due to the presence of the  $T_d^*$  phase. On cooling, for MT1, MT2, and MWT1, the rise in intensity near  $(2, 0, 2.5)$  is observed to be due to the presence of V-shape diffuse scattering; for MWT2 and MWT3, this V-shaped diffuse scattering is not clearly seen, though some increase in diffuse scattering near  $(2, 0, 2.5)$  on cooling can be seen in Figures 2(c) (in the main text) and S5, accompanying a slight movement of the  $1T'$  Bragg peaks toward  $(2, 0, 2.5)$  (ambiguous in the MWT2 data, but clear for MWT3). For MWT4 on warming, a slight

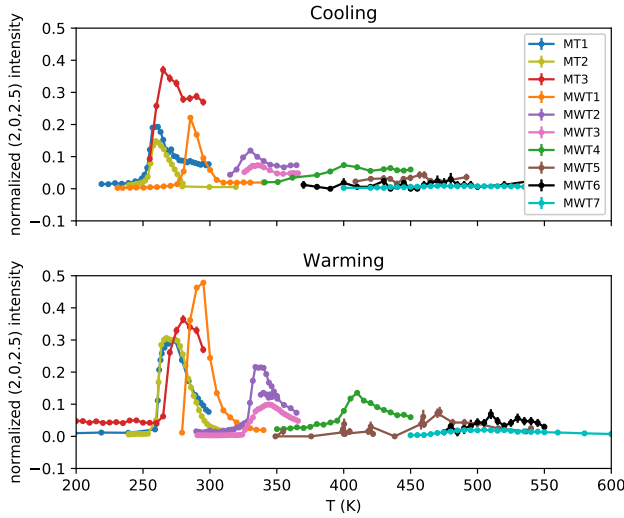

FIG. S7. Neutron scattering intensity averaged near  $(2, 0, 2.5)$  upon cooling and warming. The plotted intensities are averages of intensity along  $(2, 0, L)$  within  $2.45 \leq L \leq 2.55$ , and normalized such that intensity averaged near  $(2, 0, 3)$  is unity in the  $T_d$  phase (i.e., normalized in the same manner as for Fig. 4(a,b) of the main text.)

increase in  $(2, 0, 2.5)$  intensity is due to diffuse scattering present near 410 K, with the remaining intensity rise likely due to the averaging including the edges of the  $1T'$  peaks. No clear shift in intensity near the transition can be seen in MWT4 on cooling, or in MWT5, MWT6 or MWT7 on warming or cooling.

- 
- [1] S. M. Oliver, R. Beams, S. Krylyuk, I. Kalish, A. K. Singh, A. Bruma, F. Tavazza, J. Joshi, I. R. Stone, S. J. Stranick, A. V. Davydov, and P. M. Vora, “The structural phases and vibrational properties of  $\text{Mo}_{1-x}\text{W}_x\text{Te}_2$  alloys,” *2D Mater.* **4**, 045008 (2017).
  - [2] Y-Y. Lv, L. Cao, X. Li, B-B. Zhang, K. Wang, B. Pang, L. Ma, D. Lin, S-H. Yao, J. Zhou, Y. B. Chen, S-T. Dong, W. Liu, M-H. Lu, Y. Chen, and Y-F. Chen, “Composition and temperature-dependent phase transition in miscible  $\text{Mo}_{1-x}\text{W}_x\text{Te}_2$  single crystals,” *Sci. Rep.* **7**, srep44587 (2017).
  - [3] D. L. Bish and J. E. Post, *Modern Powder Diffraction* (Mineralogical Society of America, 1989).
  - [4] Y. Luo, H. Li, Y. M. Dai, H. Miao, Y. G. Shi, H. Ding, A. J. Taylor, D. A. Yarotski, R. P. Prasankumar, and J. D. Thompson, “Hall effect in the extremely large magnetoresistance semimetal  $\text{WTe}_2$ ,” *Appl. Phys. Lett.* **107**, 182411 (2015).
  - [5] Y. Wu, N. H. Jo, M. Ochi, L. Huang, D. Mou, S. L. Bud’ko, P. C. Canfield, N. Trivedi, R. Arita, and A. Kaminski, “Temperature-Induced Lifshitz Transition in  $\text{WTe}_2$ ,” *Phys. Rev. Lett.* **115**, 166602 (2015).
  - [6] T. Zandt, H. Dwelk, C. Janowitz, and R. Manzke, “Quadratic temperature dependence up to 50 K of the resistivity of metallic  $\text{MoTe}_2$ ,” *J. Alloys Compd. Proceedings of the 15th International Conference on Solid Compounds of Transition Elements*, **442**, 216–218 (2007).
  - [7] D. Rhodes, R. Schönmann, N. Aryal, Q. Zhou, Q. R. Zhang, E. Kampert, Y.-C. Chiu, Y. Lai, Y. Shimura, G. T. McCandless, J. Y. Chan, D. W. Paley, J. Lee, A. D. Finke, J. P. C. Ruff, S. Das, E. Manousakis, and L. Balicas, “Bulk Fermi surface of the Weyl type-II semimetallic candidate  $\gamma\text{-MoTe}_2$ ,” *Phys. Rev. B* **96**, 165134 (2017).
  - [8] S. Cho, S. H. Kang, H. S. Yu, H. W. Kim, W. Ko, S. W. Hwang, W. H. Han, D-H. Choe, Y. H. Jung, K. J. Chang, Y. H. Lee, H. Yang, and S. W. Kim, “Te vacancy-driven superconductivity in orthorhombic molybdenum ditelluride,” *2D Mater.* **4**, 021030 (2017).
  - [9] D. Santos-Cottin, E. Martino, F. Le Mardelé, C. Witteveen, F. O. von Rohr, C. C. Homes, Z. Rukelj, and Ana Akrap, “Low-energy excitations in type-II Weyl semimetal  $T_d\text{-MoTe}_2$  evidenced through optical conductivity,” *Phys. Rev. Mater.* **4**, 021201 (2020).
  - [10] C. C. Homes, M. N. Ali, and R. J. Cava, “Optical properties of the perfectly compensated semimetal  $\text{WTe}_2$ ,” *Phys. Rev. B* **92**, 161109(R) (2015).
  - [11] S. I. Kimura, Y. Nakajima, Z. Mita, R. Jha, R. Higashinaka, T. D. Matsuda, and Y. Aoki, “Optical evidence of the type-II Weyl semimetals  $\text{MoTe}_2$  and  $\text{WTe}_2$ ,” *Phys. Rev. B* **99**, 195203 (2019).
  - [12] S. Paul, S. Karak, M. Mandal, A. Ram, S. Marik, R. P. Singh, and S. Saha, “Controllable switching of the topological phases of  $1T'\text{-MoTe}_2$  investigated by Raman scattering,” *arXiv:1910.09996 [cond-mat]* (2019), arXiv: 1910.09996.
  - [13] C. Heikes, I-Lin Liu, T. Metz, C. Eckberg, P. Neves, Y. Wu, L. Hung, P. Piccoli, H. Cao, J. Leao, J. Paglione, T. Yildirim, N. P. Butch, and W. Ratcliff, “Mechanical control of crystal symmetry and superconductivity in Weyl semimetal  $\text{MoTe}_2$ ,” *Phys. Rev. Mater.* **2**, 074202 (2018).
  - [14] J. Yang, J. Colen, J. Liu, M. C. Nguyen, G-W. Chern, and D. Louca, “Elastic and electronic tuning of magnetoresistance in  $\text{MoTe}_2$ ,” *Sci. Adv.* **3**, eaao4949 (2017).

- [15] C. Cao, X. Liu, X. Ren, X. Zeng, K. Zhang, D. Sun, S. Zhou, Y. Wu, Y. Li, and J-H. Chen, “Barkhausen effect in the first order structural phase transition in type-II Weyl semimetal  $\text{MoTe}_2$ ,” *2D Mater.* **5** (2018), 10.1088/2053-1583/aae0de.
- [16] Y. Qi, P. G. Naumov, M. N. Ali, C. R. Rajamathi, W. Schnelle, O. Barkalov, M. Hanfland, S-C. Wu, C. Shekhar, Y. Sun, V. Süß, M. Schmidt, U. Schwarz, E. Pippel, P. Werner, R. Hillebrand, T. Förster, E. Kampert, S. Parkin, R. J. Cava, C. Felser, B. Yan, and S. A. Medvedev, “Superconductivity in Weyl semimetal candidate  $\text{MoTe}_2$ ,” *Nat. Commun.* **7**, 11038 (2016).
